# Supplementary material for: Topology and geometry optimization of grid-shells under self-weight loading
Source: arXiv:2505.08645 source file (2025-05-13)
Supplement: Supplementary file 1 [file Supplementary.pdf]

# Supplementary Material to: Topology and geometry optimization of grid-shells under self-weight loading

Helen E Fairclough, Karol Bołbotowski,  
Linwei He, Andrew Liew, Matthew Gilbert

May 13, 2025

This document provides additional proofs to support the manuscript ‘Topology and geometry optimization of grid-shells under self-weight loading’. Equation numbers in this document are prefixed with S; references to equations without this prefix refer to equations in the main manuscript.

## S1 Proof that downwards loads always result in gridshell solutions

Within this section, it is assumed than any vertical loads act in a downwards direction, i.e.  $\mathbf{f}_z \leq \mathbf{0}$

Assume that (22) does not hold, i.e. there is a non-empty *critical subset* of nodes at which  $w = \frac{1}{\rho g}$  (the inequality  $w \leq \frac{1}{\rho g}$  is guaranteed by the linear constraints (21c), (21d)). The goal is now to put forward a modified dual feasible solution  $\mathbf{u}, \tilde{\mathbf{w}}, \tilde{\mathbf{g}}_1, \tilde{\mathbf{g}}_2, \tilde{\mathbf{g}}_3$  such that, for every node in the critical subset,

$$\tilde{w} = w - \delta = \frac{1}{\rho g} - \delta \quad (\text{S1})$$

for a strictly positive  $\delta > 0$ , while  $\tilde{w} = w$  outside of the critical subset. If feasibility can be showed for the properly modified  $\tilde{\mathbf{g}}_1, \tilde{\mathbf{g}}_2, \tilde{\mathbf{g}}_3$ , then the modified quintuple is also optimal. Indeed, since  $\tilde{\mathbf{w}} \leq \mathbf{w}$  and  $\mathbf{f}_z \leq \mathbf{0}$ , the dual objective does not decrease after the forgoing modification. Meanwhile, clearly,  $\tilde{\mathbf{w}} < \frac{1}{\rho g}$ .

To facilitate the feasibility,  $\delta$  must be sufficiently small. It turns out it is enough to take

$$\delta = \min \left\{ \min_{g_{1,i} > 0} \frac{4 \sin \bar{l}_i}{\cos^2 l_i} g_{1,i}, \min_{g_{2,i} > 0} \frac{4 \sin \bar{l}_i}{\cos^2 l_i} g_{2,i} \right\}. \quad (\text{S2})$$

Namely, the minima above run through only those elements  $i$  for which  $g_{1,i}$  or  $g_{2,i}$  are strictly positive. The modifications  $\tilde{\mathbf{g}}_1, \tilde{\mathbf{g}}_2, \tilde{\mathbf{g}}_3$  for each element depends on whether its endpoints lie in the critical subset.

If neither of the endpoints is critical then  $\tilde{g}_1 = g_1$ ,  $\tilde{g}_2 = g_2$ ,  $\tilde{g}_3 = g_3$  (we omit the index  $i$  in the sequel).

If only one endpoint is critical, say  $A$ , then put

$$\tilde{g}_1 = \frac{\delta}{\sin \bar{l}}, \quad \tilde{g}_2 = g_2, \quad \tilde{g}_3 = -\frac{\cos \bar{l} \delta}{\sqrt{2} \sin \bar{l}}. \quad (\text{S3})$$

Observe that  $g_2 > 0$  and  $g_1 = g_3 = 0$  in this case. Evaluating the updated dual conic constraint  $2\tilde{g}_1\tilde{g}_2 \geq \tilde{g}_3^2$  for this element yields

$$2\frac{\delta}{\sin \bar{l}}g_2 \geq \frac{\cos^2 \bar{l}}{2\sin^2 \bar{l}}\delta^2 \quad (\text{S4})$$

Thanks to the choice of  $\delta$  in (S2) it is satisfied. If  $B$  is the node that is critical, then the only change is that  $\tilde{g}_1 = g_1$ ,  $\tilde{g}_2 = \frac{\delta}{\sin \bar{l}}$ .

Finally, assume that both endpoints are critical, and  $g_1 = g_2 = g_3 = 0$  as a result. Then, take

$$\tilde{g}_1 = \tilde{g}_2 = \frac{\delta}{\sin \bar{l}}, \quad \tilde{g}_3 = -\frac{\sqrt{2} \cos \bar{l} \delta}{\sin \bar{l}}. \quad (\text{S5})$$

The new dual conic constraint now reads

$$2\frac{\delta}{\sin \bar{l}}\frac{\delta}{\sin \bar{l}} \geq \frac{\cos^2 \bar{l}}{2\sin^2 \bar{l}}\delta^2, \quad (\text{S6})$$

which simplifies to  $\delta^2 \geq \cos^2 \bar{l} \delta^2$ , and, thus, it is trivially true for any  $\delta$ .

One verifies easily that the linear constraints (21c), (21d) are guaranteed to hold for the modified variables thanks to the choice of  $\tilde{\mathbf{g}}_1$ ,  $\tilde{\mathbf{g}}_2$ , respectively. The constraint (21b) is met thanks to the choice of  $\tilde{\mathbf{g}}_3$ . Indeed, it can be checked that

$$\mathbf{C}\tilde{\mathbf{g}}_1 + \mathbf{C}\tilde{\mathbf{g}}_2 + \sqrt{2}\tilde{\mathbf{g}}_3 = \mathbf{C}\mathbf{g}_1 + \mathbf{C}\mathbf{g}_2 + \sqrt{2}\mathbf{g}_3. \quad (\text{S7})$$

Admissibility of  $\mathbf{u}, \tilde{\mathbf{w}}, \tilde{\mathbf{g}}_1, \tilde{\mathbf{g}}_2, \tilde{\mathbf{g}}_3$  is thus shown, and its optimality follows.

Observe that if  $f_z < 0$  for a node in the critical subset, then the above modification produces a strict improvement of the objective function. This leads to a contradiction: the original quintuple  $\mathbf{u}, \mathbf{w}, \mathbf{g}_1, \mathbf{g}_2, \mathbf{g}_3$  cannot be optimal. Therefore,  $w < \frac{1}{\rho g}$  must hold for the nodes with  $f_z < 0$ , i.e. downwards loads must produce solutions with  $w < \frac{1}{\rho g}$ .

## S2 Problems with general loading

To prove the required properties of optimal solutions for problems with general loading, grid-shell and counterweight regions are required. Nodes are denoted as being in a grid-shell or counterweight region based on the observed optimal values of  $w$ , i.e. can only be identified after the problem has been solved.

$$w_i < \frac{1}{\rho g} \quad \forall i \text{ in a grid-shell region} \quad (\text{S8})$$

$$w_i = \frac{1}{\rho g} \quad \forall i \text{ in a counterweight region} \quad (\text{S9})$$

Elements are defined as being in a region if both end-nodes are within that region type. Elements connecting nodes of different region types will be referred to as transition elements.

*Proof of property (SI):* Without loss of generality, transition elements will be labeled so that node A is in the grid-shell region and node B is in the counterweight region. By definition, we have  $w_B = \frac{1}{\rho g}$ , and so by the dual constraint,  $g_2 = 0$ . Then by the dual cone constraint  $g_3 = 0$ . At node A, by definition  $w_A < \frac{1}{\rho g}$ , and so  $g_1 > 0$ . The complementary slackness condition (B.6) now becomes  $t_1 g_1 + 0 + 0 = 0$ , implying that  $t_1 = 0$ . Therefore by the primal conic constraint  $t_3 = 0$  and finally  $s = 0$ , giving the property (SI).

*Proof that there are no lumped masses within gridshell regions:* One possibility remains to be proven to prove that the procedure in section 3.2.2 applies exactly to grid-shell regions within solutions that also contain counterweight regions. Specifically, that the grid-shell region will not contain a lumped mass associated with an end of a transition element.

For transition elements (SI) requires  $s = 0$ , so the element does not exist and global compatibility is irrelevant, i.e. (15), (16) are trivially satisfied as  $0 = 0$ .

It need only be shown that there is no lumped mass at node A, being the node in the grid-shell region. The proof follows from that of (SI) above, which showed that  $t_1 = 0$  and  $s = 0$ . The definition of  $t_1 = \sin \bar{l} q_A + \cos \bar{l} s$  then implies this element must also have  $q_A = 0$ , i.e. there is no lumped mass contribution at the node in the grid-shell region, completing the proof. Note that this logic does not preclude the possibility of  $q_B > 0$ , i.e. this element having a lumped mass contribution at the end-point in the counterweight region.

*Proof of property (SII):* The crucial steps for this property are structural, in demonstrating a feasible physical realization. This will be shown for a problem consisting entirely of counterweight region. This does not result in loss of generality as property (SI) allows for decomposition of the problem into grid-shell and counterweight regions.

The solution in a counterweight region is highly degenerate. For an element in the counterweight region,  $w_A = w_B = \frac{1}{\rho g}$ , and hence  $g_1 = g_2 = 0$ , and from dual feasibility  $g_3 = 0$ . Thus the complementary slackness condition is trivially satisfied. The strong duality theorem can be stated for this problem as

$$\frac{1}{\rho g} \mathbf{1}^T (\mathbf{q}_A + \mathbf{q}_B) = \mathbf{f}_z^T \mathbf{w} + \mathbf{f}_{xy}^T \mathbf{u}. \quad (\text{S10})$$

From the vertical equilibrium constraint (20c), taking a sum over all rows gives  $\mathbf{1}^T (\mathbf{q}_A + \mathbf{q}_B) = \mathbf{1}^T \mathbf{f}_z$ , noting that the structure of  $\mathbf{D}_A$  and  $\mathbf{D}_B$  mean that each force is counted exactly once. Recalling that by definition  $\mathbf{w} = \frac{1}{\rho g} \mathbf{1}$ , the strong duality condition now furnishes that  $\mathbf{f}_{xy}^T \mathbf{u} = 0$ . Taking  $\mathbf{u} = \mathbf{0}$  therefore gives an optimal solution, which also satisfies (21b) with equality (i.e. we may have non-zero values in  $\mathbf{s}$  without compromising complementary slackness).

Therefore, any set of  $\mathbf{q}_A, \mathbf{q}_B, \mathbf{s}$  that satisfy primal feasibility can form a valid optimal solution. The physical interpretation of this is that we are using the material now principally for its weight, thus any configuration with the correct weight distribution is equally valid.

In the most common case where  $\mathbf{f}_{xy} = 0$ , horizontal equilibrium can be assured with  $\mathbf{s} = 0$ . Thus, even if horizontal supports have allowed for some non-zero elements in the counterweight regions of  $\mathbf{s}$ , then there is an equally-optimal solution of just lumped masses. Values of these can be obtained by summing the relevant  $q$  values at each node, and will be equal to the upwards load at that point. In this case, clearly the choice of elevation is arbitrary and independent for each lumped mass. Figure S1 gives an example of such a case, where counterweights are shown as spheres resting on the plane  $z = 0$ .

With non-zero values in  $\mathbf{f}_{xy}$ , a feasible solution is possible only if there is a feasible solution to (20b) and  $\mathbf{s} \geq \mathbf{0}$ . These constraints essentially define a standard 2D weightless truss ground structure problem, for the in-plane forces. Infeasibility (of both the equivalent truss problem and of the problem (20)) will result if the overall applied forces are unbalanced, connectivity is insufficient to obtain a valid structure, or the structure would be required to carry tensile forces. Assuming a feasible  $\mathbf{s}$  has been obtained, it remains to demonstrate how the catenary elements implied by the nonzero  $\mathbf{s}$  values can be realized in the absence of a determined elevation function.

The most reliable approach is to solve an auxiliary optimization problem, in the form of (20) for the sub-set of elements in counterweight regions with  $s > 0$ , but with the addition of a single, vertical only support at a point. Primal feasibility of this new problem is essentially the same as previous; the new reaction at the removed degree of freedom must have the same value as the lumped mass previously present there to maintain the equilibrium. Note that there will generally be multiple possible sets of elevation functions, the point chosen as support will lead to a preference for reaction force (lumped mass) being used there and the structural mass of the elements used elsewhere. Nonetheless, the solution here provides one relative set of feasible (relative) elevations for the original problem. To transfer back to the original problem, note that changing the support point back to a counterweight allows an arbitrary, simultaneous translation of all the elevations. The reaction force in the auxiliary problem should also be added back in to the lumped masses at that node.

As shown in Figure S2, this approach can cause excessive variances in elevation to ensure that all elements are fully utilized, this is a consequence of properties (II) and (III) which are reinstated by transitioning to the grid-shell problem.

A less universal, but more practical approach is to suggest a relative set of elevations (e.g. all points at equal elevation) and then seek a feasible set of variables directly. Figure S2 shows that this can give more interpretable solutions, although it should be noted that not all elevations will be possible in all cases (e.g. the solution in Figure S2d is not possible if the upwards component of force is removed on the rear node, but the solution in Figure S2b is feasible and unchanged except for reducing the size of the lumped mass at that point).

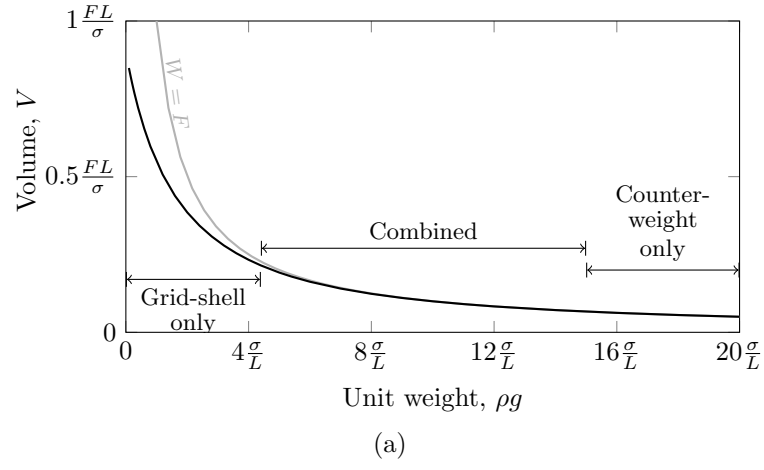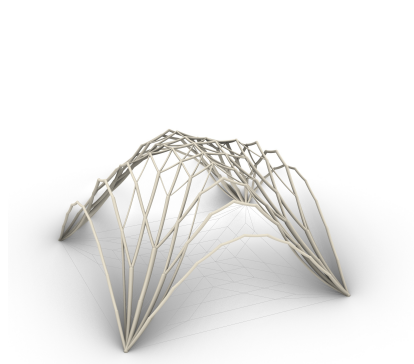

(b)  $\rho g = 2 \frac{\sigma}{L}$

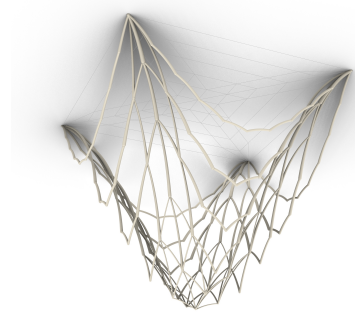

(c)  $\rho g = 4 \frac{\sigma}{L}$

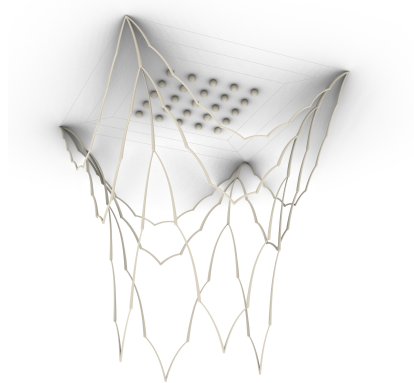

(d)  $\rho g = 6 \frac{\sigma}{L}$

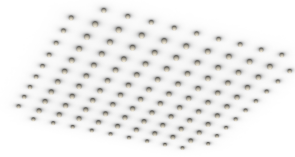

(e)  $\rho g = 16 \frac{\sigma}{L}$

Figure S1: Square domain with distributed, upwards load and point supports. (a) Optimal volumes for varying levels of self-weight. (b)-(e) selected optimal structures.

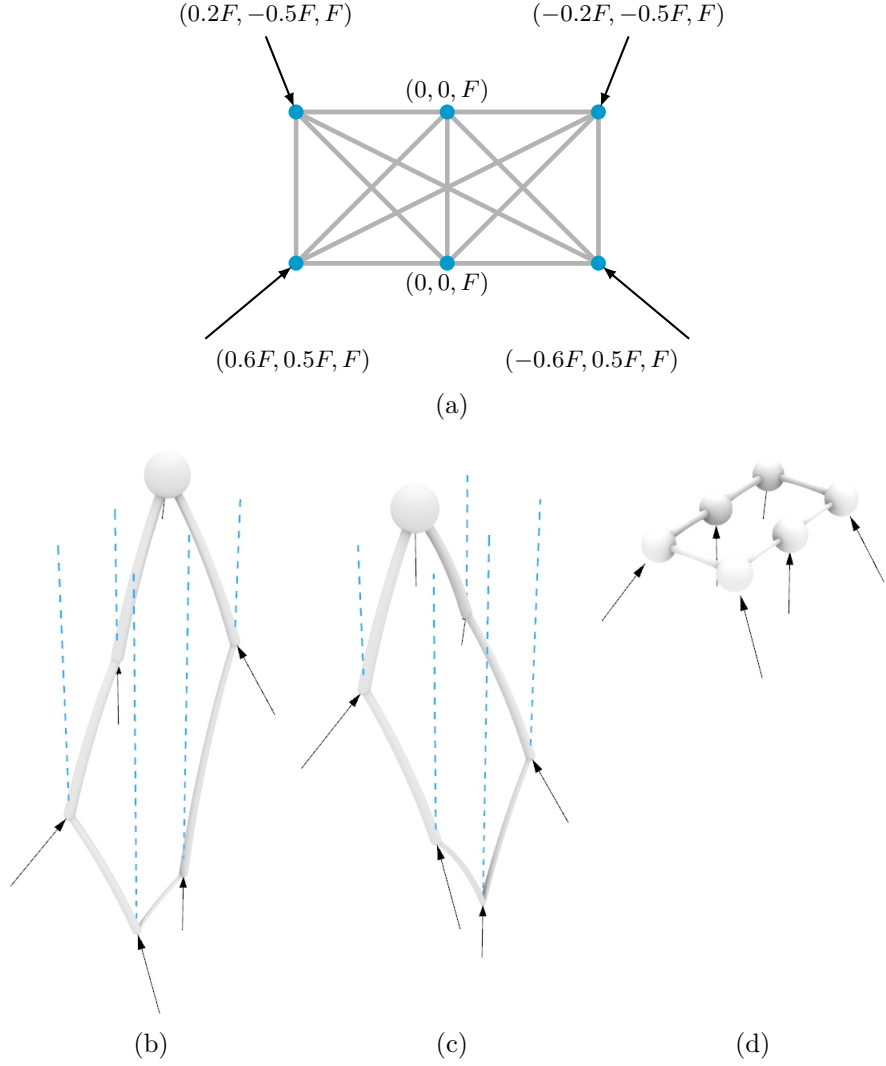

Figure S2: Reconstruction of elevations for counterweight regions with horizontal forces. (a) Problem specification indicating applied loads. Note that no supported points are specified. The material has  $\rho g = 0.6 \frac{\sigma}{L}$ . (b) and (c) Structures found by setting one point as a support, then replacing the support force with a counterbalancing lumped mass. (d) Structure found by hypothesising equal elevations at all nodes, then constructing a compatible set of elements and lumped masses. Note that (b), (c) and (d) are all equally optimal, having volume  $V = 10 \frac{FL}{\sigma}$ , such that  $W = \rho g V = 6F$ , i.e. equal to the upward force.
